# Supplementary material for: Dr.Credit: Rubric-Grounded Process Credit Assignment for Deep Research Agents
Source: arXiv:2609.34296 source file (2026-09-28)
Supplement: Supplementary file 1 [file prompt_setup.tex]

% Load once in the preamble, before \begin{document}.
% The AIbox title/body/divider design follows the supplied WikiSeeker appendix.
\RequirePackage[T1]{fontenc}
\RequirePackage{textcomp}
\RequirePackage{xcolor}
\RequirePackage{listings}
\RequirePackage{tcolorbox}
\RequirePackage{placeins}
\tcbuselibrary{breakable}

\definecolor{rcpromptgray}{gray}{0.95}
\definecolor{rcpromptblue}{RGB}{70,130,180}
\providecommand{\RCPromptVariableStyle}{\color{rcpromptblue}\bfseries}
\providecommand{\RCPromptVariable}[1]{{\RCPromptVariableStyle\{#1\}}}
\lstdefinestyle{rcprompt}{
  basicstyle=\ttfamily\fontsize{7.5pt}{8.5pt}\selectfont,
  frame=none,
  breaklines=true,
  breakatwhitespace=false,
  breakindent=0pt,
  backgroundcolor=\color{rcpromptgray},
  numbers=none,
  xleftmargin=5pt,
  xrightmargin=3pt,
  aboveskip=3pt,
  belowskip=3pt,
  columns=fullflexible,
  keepspaces=true,
  showstringspaces=false,
  moredelim=**[is][\RCPromptVariableStyle]{(*@}{@*)},
  upquote=true,
  tabsize=2
}
\tcbset{rcpromptbox/.style={
  breakable,
  after={\par\nobreak},
  title after break={\textit{Prompt continued}},
  top=8pt,
  bottom=6pt,
  left=7pt,
  right=7pt,
  colback=white,
  colframe=black!75,
  colbacktitle=black!75,
  coltitle=white,
  fonttitle=\bfseries\fontsize{10pt}{12pt}\selectfont,
  fontupper=\fontsize{9pt}{10pt}\selectfont,
  fontlower=\fontsize{9pt}{10pt}\selectfont,
  before upper={\setlength{\parindent}{0pt}\setlength{\parskip}{0pt}\raggedright},
  before lower={\setlength{\parindent}{0pt}\setlength{\parskip}{0pt}\raggedright}
}}
% Reuse AIbox when the host paper already defines it; avoid a name collision.
\ifcsname AIbox\endcsname
\else
  \newtcolorbox{AIbox}[2][]{rcpromptbox,title=#2,#1}
\fi
\providecommand{\RCPromptRole}[1]{%
  {\color{black}\bfseries\fontsize{10pt}{12pt}\selectfont #1}\par\vspace{3pt}}

% Prompt boxes flow with their explanatory text and may continue across pages.
\makeatletter
\newenvironment{RCPromptFigure}{\par\begingroup\def\@captype{figure}}{\par\endgroup\vspace{8pt}}
\makeatother
